# Supplementary material for: Unsupervised Domain Expansion for Visual Categorization
Source: arXiv:2104.00233 source file (2021-04-01)
Supplement: Supplementary file 1 [file appendix-pseudo-code.tex]

In order to further explain the KDDE training and validation process, we prepare the pseudo-code below, which contains three algorithms, corresponding to the three steps in Fig \ref{fig:method}.
\begin{algorithm}
\caption{Training a domain-specific model $G_{s}$}\label{algorithm1}
\KwIn{($X_{s}^{train}$,$Y_{s}^{train}$),($X_{s}^{test}$,$Y_{s}^{test}$),($X_{t}^{test}$,$Y_{t}^{test}$)}
\KwOut{$\theta(G_{s})$}
Initialize {$\theta(G_{s})$} as ImageNet parameters\;
\For{$I\leftarrow 1,MAX\_EPOCH$}{
    \For{$J\leftarrow 1,MAX\_ITER$}{
        Sample $X_{s}^{train(batch)}$,$Y_{s}^{train(batch)}$ from $X_{s}^{train}$,$Y_{s}^{train}$\;
        Compute $L_{clf}$ of $G_{s}$ by $X_{s}^{train(batch)}$,$Y_{s}^{train(batch)}$\;
        Update $\theta(G_{s})$ by minimizing $L_{clf}$
        }
    }
Evaluate well-trained $G_{s}$ on source domain by $X_{s}^{test}$,$Y_{s}^{test}$\;
Evaluate well-trained $G_{s}$ on target domain by $X_{t}^{test}$,$Y_{t}^{test}$\;
Evaluate well-trained $G_{s}$ on expanded domain by \{$X_{s}^{test}$,$X_{t}^{test}$\},\{$Y_{s}^{test}$,$Y_{t}^{test}$\}
\end{algorithm}

\begin{algorithm}
\caption{Training a domain-specific model $G_{s\rightarrow t}$}\label{algorithm2}
\KwIn{($X_{s}^{train}$,$Y_{s}^{train}$),($X_{s}^{test}$,$Y_{s}^{test}$),$X_{t}^{train}$,($X_{t}^{test}$,$Y_{t}^{test}$),$\lambda$}
\KwOut{$\theta(G_{s\rightarrow t})$}
Initialize {$\theta(G_{s\rightarrow t})$} as ImageNet parameters\;
\For{$I\leftarrow 1,MAX\_EPOCH$}{
    \For{$J\leftarrow 1,MAX\_ITER$}{
        Sample $X_{s}^{train(batch)}$,$Y_{s}^{train(batch)}$ from $X_{s}^{train}$,$Y_{s}^{train}$\;
        
        Sample $X_{t}^{train(batch)}$ from $X_{t}^{train}$\;
        
        Compute $L_{clf}$ of $G_{s\rightarrow t}$ by $X_{s}^{train(batch)}$,$Y_{s}^{train(batch)}$\;
        
        Compute $L_{da}$ of $G_{s\rightarrow t}$ by $X_{s}^{train(batch)}$,$X_{t}^{train(batch)}$\;
        Update $\theta(G_{s\rightarrow t})$ by minimizing $L_{clf}+\lambda*L_{da}$
        }
    }
Evaluate well-trained $G_{s\rightarrow t}$ on source domain by $X_{s}^{test}$,$Y_{s}^{test}$\;
Evaluate well-trained $G_{s\rightarrow t}$ on target domain by $X_{t}^{test}$,$Y_{t}^{test}$\;
Evaluate well-trained $G_{s\rightarrow t}$ on expanded domain by \{$X_{s}^{test}$,$X_{t}^{test}$\},\{$Y_{s}^{test}$,$Y_{t}^{test}$\}
\end{algorithm}

\begin{algorithm}
\caption{Training a domain-invariant model $G_{s+t}$}\label{algorithm3}
\KwIn{$X_{s}^{train}$,($X_{s}^{test}$,$Y_{s}^{test}$),$X_{t}^{train}$,($X_{t}^{test}$,$Y_{t}^{test}$),$\theta(G_{s})$,$\theta(G_{s\rightarrow t})$}
\KwOut{$\theta(G_{s+t})$}
Restore $G_{s}$ from $\theta(G_{s})$\;
Restore $G_{s\rightarrow t}$ from $\theta(G_{s\rightarrow t})$\;
\For{$I\leftarrow 1,MAX\_EPOCH$}{
    \For{$J\leftarrow 1,MAX\_ITER$}{
        Sample $X_{s}^{train(batch)}$ from $X_{s}^{train}$\;
        
        Sample $X_{t}^{train(batch)}$ from $X_{t}^{train}$\;
        
        Compute $L_{kd}^{s}=KL(P(G_{s}(X_{s}^{train(batch)})||P(G_{s+t}(X_{s}^{train(batch)}))$ \;
        
        Compute $L_{kd}^{t}=KL(P(G_{s\rightarrow t}(X_{t}^{train(batch)})||P(G_{s+t}(X_{t}^{train(batch)}))$\;
        Update $\theta(G_{s+t})$ by minimizing $L_{kd}^{s}+L_{kd}^{t}$
        }
    }
Evaluate well-trained $G_{s+t}$ on source domain by $X_{s}^{test}$,$Y_{s}^{test}$\;
Evaluate well-trained $G_{s+t}$ on target domain by $X_{t}^{test}$,$Y_{t}^{test}$\;
Evaluate well-trained $G_{s+t}$ on expanded domain by \{$X_{s}^{test}$,$X_{t}^{test}$\},\{$Y_{s}^{test}$,$Y_{t}^{test}$\}
\end{algorithm}
