# Supplementary material for: Unsupervised Domain Expansion for Visual Categorization
Source: arXiv:2104.00233 source file (2021-04-01)
Supplement: Supplementary file 2 [file appendix-MCD.tex]

We would like to clarify that the proposed KDDE is agnostic to the implementation of a specific UDA model it uses. 
Therefore, we compare KDDE(MCD) with MCD to prove this point. 
We take two tasks C$\rightarrow$A P$\rightarrow$R of Office-Home as examples. 
We train all extractors to start with ResNet-50 backbone pre-trained on ImageNet. 
SGD is used for training, with a momentum of 0.9 and weight decay of 0.0005. 
The initial learning rate is empirically set to 0.001 for MCD and 0.005 for KDDE(MCD). 
The learning rate is decayed by 0.1 every 30 epochs. 
In Stage two of MCD, we set $\lambda$ as 10 for maximizing the loss of target data discrepancy between two classifiers. 
In Stage three of MCD, we repeat three times to minimizing the loss of target data discrepancy between two classifiers. 
According to the experimental results in Table \ref{tab:MCD}, KDDE(MCD) further improves the performance of MCD. 

\begin{table}[tbh!]
    \centering
    \caption{\textbf{Comparison of MCD and KDDE(MCD)}. we get three times results to get average value and standard deviation.} 
    \label{tab:MCD}
    \resizebox{0.98\textwidth}{!}{
    \begin{tabular}{|c|c|c|c|c|c|c|}
    \hline
    \multirow{2}{*}{Model} & \multicolumn{3}{c|}{C$\rightarrow$A}           & \multicolumn{3}{c|}{P$\rightarrow$R}           \\ \cline{2-7} 
                           & C              & A              & C+A            & P              & R              & P+R            \\ \hline
    MCD                    & 77.53$\pm$0.66 & 51.90$\pm$0.96 & 64.72$\pm$0.53 & 91.45$\pm$0.32 & 70.67$\pm$0.71 & 81.06$\pm$0.51 \\ \hline
    KDDE(MCD)              & 79.20$\pm$0.35 & 56.33$\pm$0.65 & 67.77$\pm$0.49 & 92.25$\pm$0.16 & 73.91$\pm$0.10 & 83.08$\pm$0.04 \\ \hline
    \end{tabular}
    }
\end{table}
