# Supplementary material for: Unsupervised Domain Expansion for Visual Categorization
Source: arXiv:2104.00233 source file (2021-04-01)
Supplement: Supplementary file 3 [file appendix-cross-domain.tex]

To further explain the precise effect of knowledge distillation at the intermediate features space, we visualize the cross-domain retrieval results and compute top-k mean accuracy on C$\rightarrow$A and P$\rightarrow$R tasks of Office-Home. In Table \ref{tab:cross-domain}, top-k accuracy means probability that the top closest k target(source) neighbors and the source(target) retrieved data are the same class.  We compute top 1,5,10 mean accuracy to show the class clusters become more compact after knowledge distillation. In Fig. \ref{fig:cross-domain}, we draw one source(target) image's top-5 target(source) neighbors in feature space for three models. We can clearly observe, compared with the DA model and source-only model, neighbors after KDDE are more similar to the retrieved data. 

\begin{table*}[tbh!]
	\caption{\textbf{Accuracy of cross domain retrieval}. "S retrieve T" means that source data retrieves target neighbors. "T retrieve S" means the opposite.}
	\label{tab:cross-domain}
	\centering
	\resizebox{0.98\textwidth}{!}
	{
		\begin{tabular}{|l|c|c|c|c|c|c|c|c|c|c|c|c|}
		\hline
		\multicolumn{1}{|c|}{\multirow{3}{*}{Model}} & \multicolumn{6}{c|}{C$\rightarrow$A} & \multicolumn{6}{c|}{P$\rightarrow$R} \\ \cline{2-13} 
		\multicolumn{1}{|c|}{} & \multicolumn{3}{c|}{S retrieve T} & \multicolumn{3}{c|}{T retrieve S} & \multicolumn{3}{c|}{S retrieval T} & \multicolumn{3}{c|}{T retrieval S} \\ \cline{2-13} 
		\multicolumn{1}{|c|}{} & top1 & top5 & top10 & top1 & top5 & top10 & top1 & top5 & top10 & top1 & top5 & top10 \\ \hline
		ResNet-50 & 56.73 & 48.14 & 40.49 & 40.40 & 37.16 & 35.22 & \textbf{81.34} & 75.97 & 72.14 & \textbf{68.67} & 63.86 & 61.93 \\ \hline
		DDC & 53.41 & 43.54 & 35.78 & 44.26 & 40.11 & 37.42 & 76.15 & 70.88 & 66.08 & 66.52 & 63.54 & 60.54 \\ \hline
		KDDE(DDC) & \textbf{59.51} & \textbf{50.10} & \textbf{42.69} & \textbf{46.28} & \textbf{43.62} & \textbf{41.44} & 80.03 & \textbf{76.66} & \textbf{72.89} & 66.72 & \textbf{66.56} & \textbf{64.83} \\ \hline
		\end{tabular}
	}
\end{table*}
	
\begin{figure*}[tbh!]
	\centering
	\includegraphics[width=\textwidth]{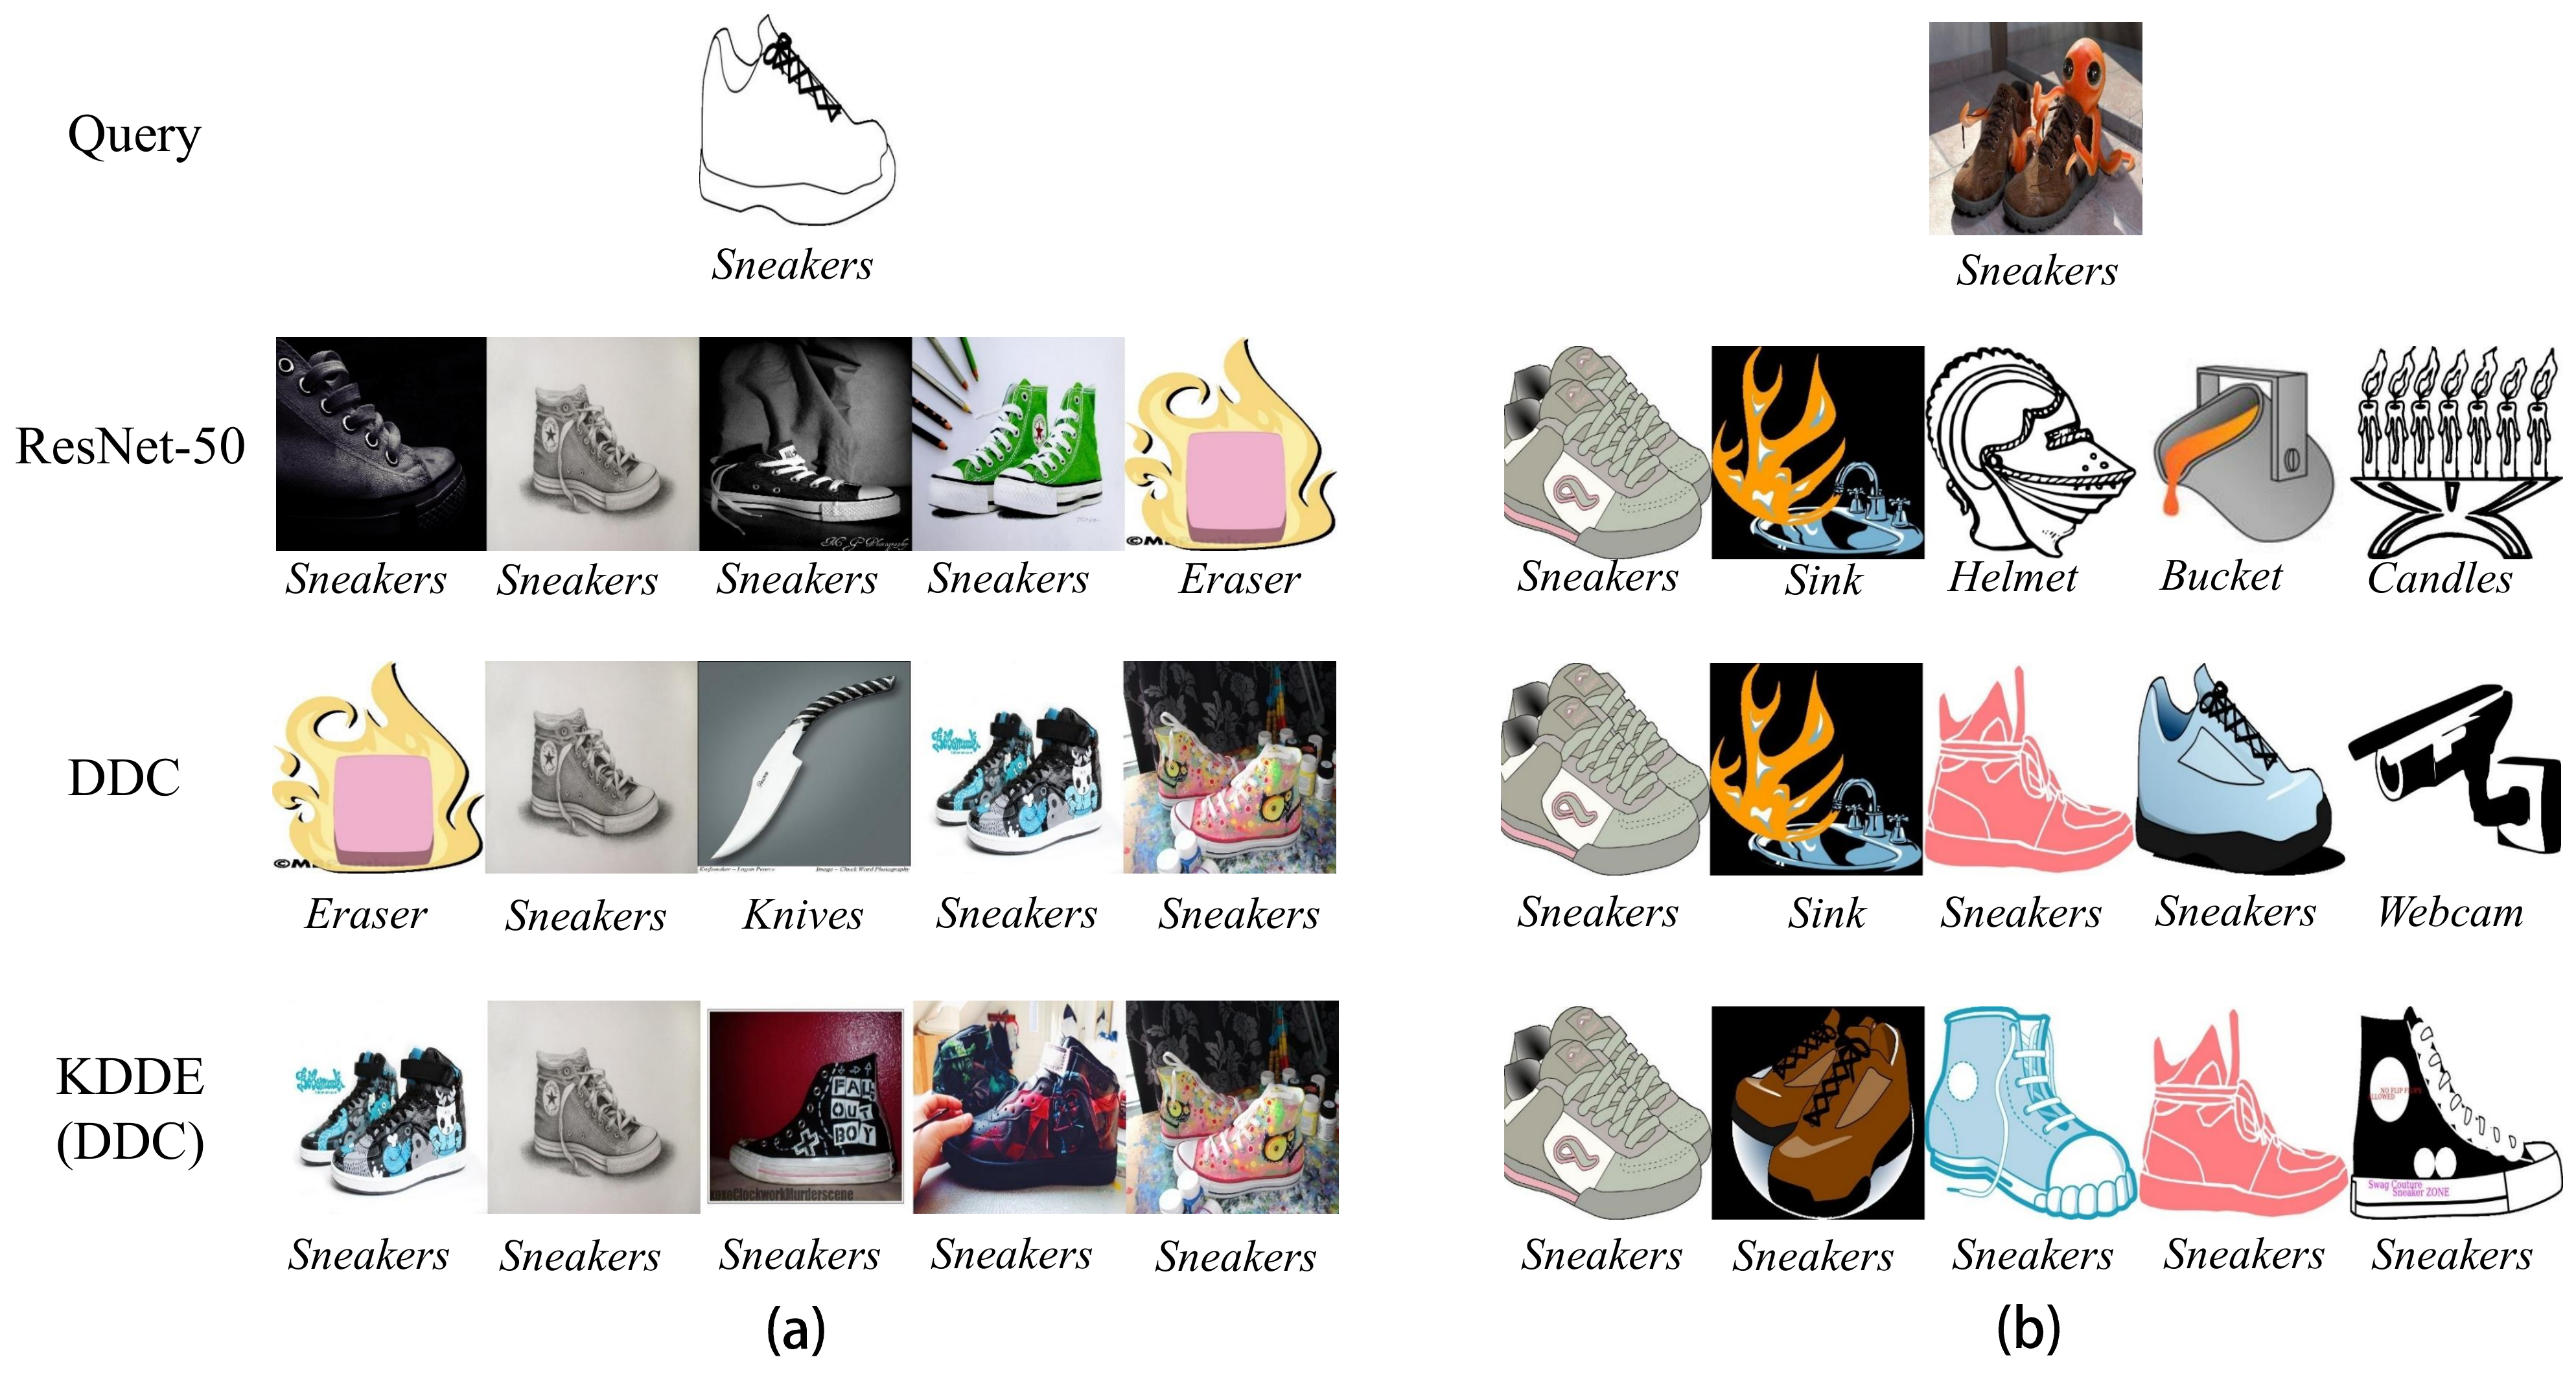}
	\caption{\textbf{Visualization of cross domain retrieval}. "Query" means the retrieved domain Clipart(Art) data. Top-5 domain Art(Clipart) neighbors are ranked by the euclidean distance with the retrieved data in feature space.}
	\label{fig:cross-domain}
	% \subfigure[\textbf{Clipart$\rightarrow$Art}]{
	% 	\includegraphics[width=\columnwidth]{diagrams/cross-domain-C2A}
	% 	\label{fig:crossdomain-C2A}
	% }
	% \subfigure[\textbf{Product$\rightarrow$Real\_World}]{
	% 	\includegraphics[width=\columnwidth]{diagrams/cross-domain-P2R}
	% 	\label{fig:crossdomain-P2R}
	% }
	% \subfigure[\textbf{Real\_World$\rightarrow$Clipart}]{
	% 	\includegraphics[width=\columnwidth]{diagrams/cross-domain-R2C}
	% 	\label{fig:crossdomain-R2C}
	% }
	% \caption{\textbf{xx}.yy. }
	% \label{fig:crossdomain}
\end{figure*}
