# Supplementary material for: Unsupervised Domain Expansion for Visual Categorization
Source: arXiv:2104.00233 source file (2021-04-01)
Supplement: Supplementary file 4 [file appendix-different-lambdas.tex]

One concern that is likely to arise is whether we can obtain a more generalized model to perform both source and target well by tuning the trade-off parameter $\lambda$ of $L_{clf}$ and $L_{da}$.
The $\lambda$ of the UDA is usually optimal for UDA tasks.
So, changing the $\lambda$ , we cannot get a better model on the target domain, while our method on target domain is better than UDA models. 
As for the performance on source domain when changing the $\lambda$, it has never been discussed before and our UDE pays attention to it.
To further address this concern, we add some experiments.
we take DDC as an example, we evaluate the model with different $\lambda$ on three tasks of OfficeHome.
In the training process, the training strategy is the same as mentioned in Section \ref{ssec:implement}.
According to the Table \ref{tab:different-lambdas}, it can be seen that different lambdas achieve the best performance in different specific tasks.
According to Fig. \ref{fig:different-lambdas}, it can be seen that the different lambda models are still not better than our distilled model.

It is worth mentioning that the DDC model with $\lambda=0$ is different from the ResNet-50 model.
In the DDC model with $\lambda=0$, although the $L_{da}$ loss will not be backpropagated, the training set of the target domain participates in the training process.
In contrast, in ResNet-50, the target domain training set is not involved in training at all.
There are BN layers in the ResNet-50 backbone that we use, which records the average and deviation of all data passing through the network. Therefore, the performance of the DDC model with $\lambda=0$ will be better than the ResNet-50 model. When $\lambda$ is set to 100, the network can't be trained.

\begin{figure}[tbh!]
  \centering
  \includegraphics[width=0.5\textwidth]{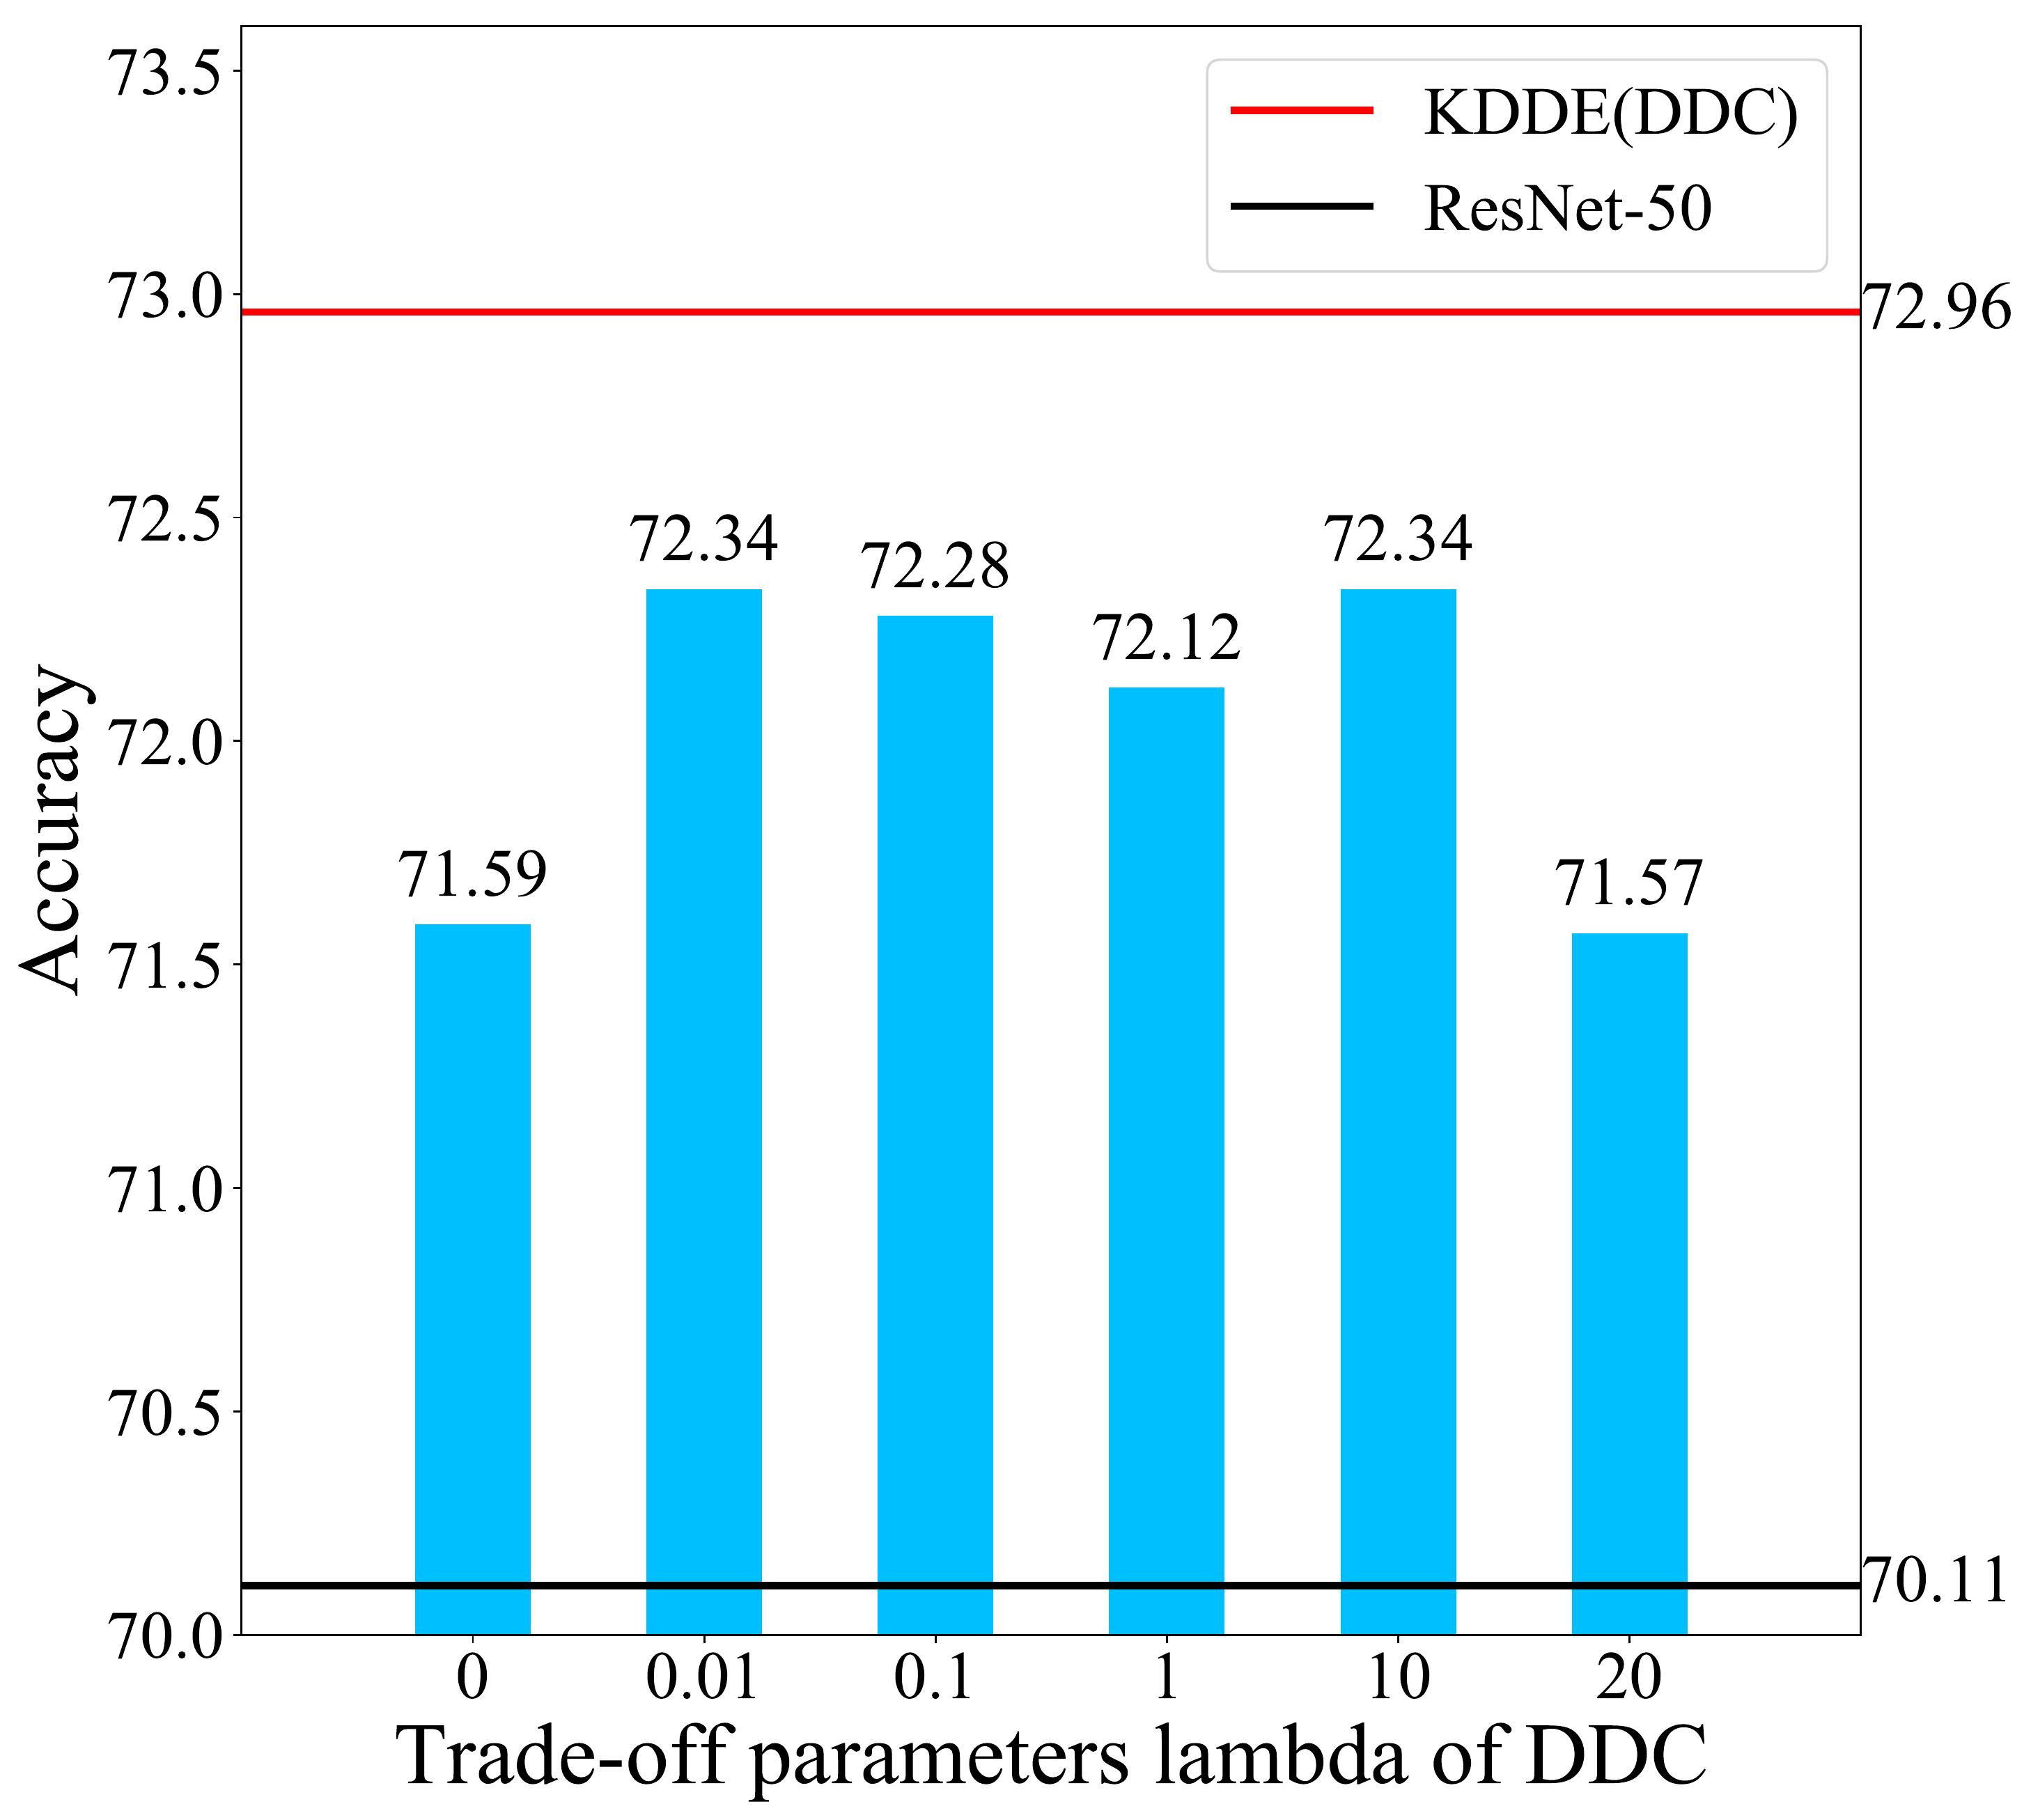}
  \caption{\textbf{Average accuracy on expanded domain for three tasks of Office-Home.} the red line means KDDE(DDC,$\lambda=10$), the black line means ResNet-50.}
  \label{fig:different-lambdas}
\end{figure}

\begin{table*}[tbh!]
    \caption{\textbf{Comparison of DDC with different lambdas and KDDE(DDC).} KDDE(DDC,$\lambda=10$) performs the best.}
	\label{tab:different-lambdas}
	\centering
	\resizebox{0.98\textwidth}{!}
	{
		\begin{tabular}{|c|c|c|c|c|c|c|c|c|c|c|c|}
			\hline
			\multicolumn{2}{|c|}{\multirow{2}{*}{Model}} & \multicolumn{3}{c|}{C$\rightarrow$A}                                                                            & \multicolumn{3}{c|}{P$\rightarrow$R}                                                                   & \multicolumn{3}{c|}{R$\rightarrow$C}                                                          & \multirow{2}{*}{\begin{tabular}[c]{@{}c@{}}Average accuracy\\ on expanded domain\end{tabular}} \\ \cline{3-11}
			\multicolumn{2}{|c|}{}                       & C                                   & A                                   & C+A                                 & P                          & R                                   & P+R                                 & R                          & C                                   & R+C                        &                                                                                                \\ \hline
			\multicolumn{2}{|c|}{ResNet-50}              & 78.91                               & 47.06                               & 62.99                               & 92.05                      & 70.31                               & 81.18                               & \textbf{84.11}             & 48.23                               & 66.17                      & 70.11                                                                                          \\ \hline
			\multicolumn{2}{|l|}{KDDE(DDC,$\lambda=10$)} & \multicolumn{1}{l|}{\textbf{80.05}} & \multicolumn{1}{l|}{\textbf{54.57}} & \multicolumn{1}{l|}{\textbf{67.31}} & \multicolumn{1}{l|}{92.67} & \multicolumn{1}{l|}{\textbf{73.36}} & \multicolumn{1}{l|}{\textbf{83.02}} & \multicolumn{1}{l|}{83.24} & \multicolumn{1}{l|}{\textbf{53.86}} & \multicolumn{1}{l|}{68.55} & \textbf{72.96}                                                                                 \\ \hline
			\multirow{7}{*}{DDC}     & $\lambda$=0       & 78.68                               & 51.55                               & 65.12                               & 92.05                      & 71.54                               & 81.80                               & 83.01                      & 52.73                               & 67.87                      & 71.59                                                                                          \\ \cline{2-12} 
									 & $\lambda$=0.01    & 79.41                               & 52.28                               & 65.85                               & 92.40                      & 72.54                               & 82.47                               & 83.56                      & 53.82                               & \textbf{68.69}             & 72.34                                                                                          \\ \cline{2-12} 
									 & $\lambda$=0.1     & 79.86                               & 52.37                               & 66.12                               & 92.58                      & 72.13                               & 82.36                               & 82.97                      & 53.77                               & 68.37                      & 72.28                                                                                          \\ \cline{2-12} 
									 & $\lambda$=1       & 79.23                               & 51.47                               & 65.35                               & \textbf{92.72}             & 73.04                               & 82.88                               & 83.42                      & 52.82                               & 68.12                      & 72.12                                                                                          \\ \cline{2-12} 
									 & $\lambda$=10      & 79.45                               & 53.26                               & 66.36                               & 92.40                      & 72.68                               & 82.54                               & 83.24                      & 53.00                               & 68.12                      & 72.34                                                                                          \\ \cline{2-12} 
									 & $\lambda$=20      & 79.23                               & 51.47                               & 65.35                               & 92.09                      & 71.27                               & 81.68                               & 83.20                      & 52.14                               & 67.67                      & 71.57                                                                                          \\ \cline{2-12} 
									 & $\lambda$=100     & 7.96                                & 2.53                                & 5.25                                & 13.50                      & 5.64                                & 9.57                                & 6.33                       & 3.41                                & 4.87                       & 6.59                                                                                           \\ \hline
			\end{tabular}
	}
\end{table*}
