# Supplementary material for: Unsupervised Domain Expansion for Visual Categorization
Source: arXiv:2104.00233 source file (2021-04-01)
Supplement: Supplementary file 5 [file appendix-kd-loss.tex]

% Please add the following required packages to your document preamble:
% \usepackage{multirow}
\begin{table}[]
  \label{tab:kd-loss}
  \caption{\textbf{Comparison of different knowledge distillation loss function.} KL is the KL divergence loss. CE is the cross entropy loss. The values are the average of the 12 tasks on Office-Home.}
  \begin{tabular}{|l|c|c|c|}
  \hline
  \multirow{2}{*}{Model} & \multicolumn{3}{c|}{Office-Home} \\ \cline{2-4} 
   & \textit{Source domain} & \textit{Target domain} & \textit{Expanded domain} \\ \hline
  ResNet-50 & \textbf{82.57} & 57.49 & 70.03 \\ \hline
  CDAN & 80.54 & 61.85 & 71.20 \\ \hline
  KDDE ($L_2$) & 79.60 & 61.77 & 70.69 \\ \hline
  KDDE (CE) & 80.78 & 63.19 & 71.99 \\ \hline
  KDDE (KL) & 81.44 & \textbf{63.90} & \textbf{72.67} \\ \hline
  \end{tabular}
\end{table}

To explore the impact of different type of knowledge distillation loss, we apply KDDE on  Office-Home. In this case, we use ResNet-50 and CDAN as the two domain-specific model. In Table \ref{tab:kd-loss}, we compare $L_2$, cross entropy (CE) and KL divergence. KL divergence is usually used to minimize the distance of two distributions. Cross entropy loss is often used in classification, where the label is hard label. In knowledge distillation, $L_2$ is usually used on feature space. As shown in Table \ref{tab:kd-loss}, KL divergence get the best performance. KDDE ($L_2$) is even lower than CDAN. Therefore, KL divergence is the suitable knowledge loss in the task.
