# Supplementary material for: Unsupervised Domain Expansion for Visual Categorization
Source: arXiv:2104.00233 source file (2021-04-01)
Supplement: Supplementary file 6 [file appendix-multi-domain.tex]

To futher study the scenario where exists multiple domain shifts, we consider single-source domain and multi-target domains experiment setting. 
If the domain adaptation model can solve data from multi-target domains, KDDE is competent to the task.
We can extend CDAN by modifying the discriminator from a two-domain classifier to a multi-domain classifier to adapt to multi-target domains. 
The multi-target CDAN is used as $G_{s \rightarrow t}$.
When training the student $G_{s+t}$, it learns from $G_s$ on the source data, and from $G_{s \rightarrow t}$ on the multi-domain target data.
To illustrate the effictiveness of KDDE on multi-domain shifts, we run experiments on Office-Home. We use one domain as source domain and the other three domains as target domains.
Result is shown in Table \ref{tab:multi-domain}.

\begin{table}[]
    \caption{\textbf{Multiple domain shift on Office-Home.} We use one domain as source domain, and the other three domains as target domains. KDDE in this table is based on CDAN.}
    \label{tab:multi-domain}
    \begin{tabular}{|l|c|c|c|c|c|}
    \hline
    \multicolumn{1}{|c|}{\multirow{2}{*}{Model}} & \multicolumn{5}{c|}{A$\rightarrow$C,P,R} \\ \cline{2-6} 
    \multicolumn{1}{|c|}{} & A & C & P & R & Avg \\ \hline
    ResNet-50                 & \textbf{75.20} & 45.23 & 57.91 & 69.35 & 61.92 \\ \hline
    CDAN(A$\rightarrow$C,P,R) & 70.64 & \textbf{50.23} & 61.35 & 67.17 & 62.35 \\ \hline
    KDDE(A$\rightarrow$C,P,R) & 72.59 & 50.14 & \textbf{63.49} & \textbf{69.49} & \textbf{63.93} \\ \hline

    \multicolumn{1}{|c|}{\multirow{2}{*}{Model}} & \multicolumn{5}{c|}{C$\rightarrow$A,P,R} \\ \cline{2-6} 
    \multicolumn{1}{|c|}{} & C & A & P & R & Avg \\ \hline
    ResNet-50                 & 78.91 & 47.06 & 57.55 & 59.65 & 60.79\\ \hline
    CDAN(C$\rightarrow$A,P,R) & 77.09 & 54.89 & 66.53 & 64.62 & 65.78 \\ \hline
    KDDE(A$\rightarrow$C,P,R) & \textbf{79.05} & \textbf{57.67} & \textbf{68.19} & \textbf{66.94} & \textbf{67.96} \\ \hline

    \multicolumn{1}{|c|}{\multirow{2}{*}{Model}} & \multicolumn{5}{c|}{P$\rightarrow$A,C,R} \\ \cline{2-6} 
    \multicolumn{1}{|c|}{} & P & A & C & R & Avg \\ \hline
    ResNet-50                 & \textbf{92.05} & 50.33 & 43.86 & 70.31 & 64.14 \\ \hline
    CDAN(P$\rightarrow$A,C,R) & 90.08 & 54.24 & 47.91 & 70.90 & 65.78 \\ \hline
    KDDE(P$\rightarrow$A,C,R) & 91.33 & \textbf{56.28} & \textbf{50.50} & \textbf{72.04} & \textbf{67.54} \\ \hline

    \multicolumn{1}{|c|}{\multirow{2}{*}{Model}} & \multicolumn{5}{c|}{R$\rightarrow$A,C,P} \\ \cline{2-6} 
    \multicolumn{1}{|c|}{} & R & A & C & P & Avg \\ \hline
    ResNet-50                 & \textbf{84.11} & 63.62 & 48.23 & 76.27 & 68.06 \\ \hline
    CDAN(R$\rightarrow$A,C,P) & 82.01 & 62.40 & 57.14 & 76.32 & 69.47 \\ \hline
    KDDE(P$\rightarrow$A,C,R) & 82.65 & 63.30 & \textbf{57.27} & \textbf{77.97} & \textbf{70.30} \\ \hline
    \end{tabular}
\end{table}
